# Supplementary material for: Benchmarking Automated Machine Learning Methods for Price Forecasting Applications
Source: arXiv:2304.14735 source file (2023-04-28)
Supplement: Supplementary file 1 [file 06-appendix.tex]

\section*{\uppercase{Appendix}}
\label{app:appendic}

\subsection*{Implementation details}
\label{app:implemantation-details}

The manual implementation of the ML methods (\textit{Polynomial Regression}, \textit{Decision Tree}, \textit{Random Forest}, \textit{Support Vector Regressor}, \textit{K-Nearest Neighbor} and \textit{AdaBoost Regressor}) require approximately 50 lines of code (LOC) on average and $13$ different libraries:

\begin{minted}[mathescape]{python}
from sklearn.pipeline import Pipeline
from sklearn.model_selection import RandomizedSearchCV
from sklearn.model_selection import GridSearchCV, KFold
from sklearn.preprocessing import PolynomialFeatures
from sklearn.linear_model import LinearRegression
from sklearn.tree import DecisionTreeRegressor
from sklearn.ensemble import RandomForestRegressor
from sklearn.ensemble import AdaBoostRegressor
from sklearn.svm import SVR
from sklearn.neighbors import KNeighborsRegressor
from sklearn.metrics import mean_squared_error
from sklearn.metrics import mean_absolute_error
from sklearn.metrics import mean_absolute_percentage_error
\end{minted}

\noindent On the other hand training and prediction with \textit{Autogluon} can be implemented within five lines of code:

\begin{minted}[mathescape]{python}
from sklearn.model_selection import train_test_split
X_train, X_test=train_test_split(df,test_size=0.2)
from autogluon.tabular import TabularPredictor
automl = TabularPredictor(label='price').fit(X_train)
predictions = automl.predict(X_test)
\end{minted}

\noindent The same holds for \textit{AutoSklearn}
\begin{minted}[mathescape]{python}
from sklearn.model_selection import train_test_split
X_train, X_test=train_test_split(df,test_size=0.2)
from autosklearn.regression import AutoSklearnRegressor
automl = AutoSklearnRegressor().fit(X_train, y_train)
predictions = automl.predict(X_test)
\end{minted}

\noindent and \textit{Flaml}
\begin{minted}[mathescape]{python}
from sklearn.model_selection import train_test_split
X_train, X_test=train_test_split(df,test_size=0.2)
from flaml import AutoML
automl = AutoML().fit(X_train = X_train, y_train = y_train)
predictions = automl.predict(X_test)
\end{minted}

%\clearpage
\subsection*{Tables}
\label{app:tables}

\begin{table*}[ht]
    \caption{\ac{ML} Hyperparameter}
    \label{table:ml-hyperparameter}
    \begin{tabular*}{\textwidth}{@{\extracolsep{\fill}}l l l }
     \toprule
     %\rowcolor{lightgray}
     Model & Hyperparameter & Values\\ [0.5ex]
     \midrule
     Polynomial Regression      & Degree            & 1,2,3,4 \\
     Decision tree              & Depth             & 0, 5, 10, 15, 20  \\
                                & Criterion         & squared\_error, absolute\_error, poisson  \\
     Random forest              & Depth             & 0, 5, 10, 15, 20  \\
                                & Criterion         & squared\_error, absolute\_error, poisson  \\
                                & Estimators        & randint(1, 200)  \\
                                & Features          & randint(1, column\_count)  \\
                                & Sample split      & randint(2, 11)  \\
                                & Bootstrap         & True, False  \\
     Support Vector Regressor   & Kernel            & Linear, poly, RBF \\
                                & C                 & 0.1, 1, 10, 100, 1000 \\
                                & Epsilon           & 1 x $10^{-5}$, 1 x $10^{-4}$, 1 x $10^{-3}$, 1 x $10^{-2}$ \\
     K-Nearest Neighbor         & N\_Neighbors      & 2, 4, 6, 8, 10 \\
                                & Weights           & Uniform, Distance \\
                                & P                 & 1, 2, 3 \\
     AdaBoost Regressor         & Estimators        & randint(1, 200) \\
     Neural Network             & Hidden Layer Size & 1, 3, 5, 7, 9 \\
                                & Learning Rate     & 1 x $10^{-3}$ \\
                                & Activation        & Relu \\
                                & Solver            & Adam \\
    \bottomrule
    \end{tabular*}
\end{table*}

    \begin{table*}[htpb]
        \caption{\ac{AutoML} configuration}
        \label{table:automl-parameter}
        \begin{tabular*}{\textwidth}{@{\extracolsep{\fill}}l l l }
         \toprule
         %\rowcolor{lightgray}
         Model                      & Parameter                 & Values\\
         \midrule
         Auto-Sklearn               & Time budget per dataset   & 300 seconds  \\
                                    & Time budget per algorithm & 30 seconds  \\
                                    & Metric                    & Mean Absolute Error \\
         AutoGluon                  & Time budget               & 300 seconds  \\
                                    & Metric                    & Mean Absolute Percentage Error  \\
         Flaml                      & Task                      & Regression  \\
                                    & Time budget               & 300 seconds  \\
                                    & Metric                    & Mean Absolute Percentage Error \\
        \bottomrule
        \end{tabular*}
    \end{table*}

\begin{table*}[htpb]
    \caption{\ac{ML} and \ac{AutoML} methods}
    \label{table:ml-automl-methods}
    %\begin{tabular*}{\textwidth}{@{\extracolsep{\fill}}l l l }
    \begin{tabular}{p{4.5cm} p{3cm} p{2cm}}
     \toprule
     %\rowcolor{lightgray}
     Model & Library & Version\\
     \midrule
     Polynomial Regression & scikit-learn & 0.24.2 \\
     Decision tree & scikit-learn & 0.24.2 \\
     Random forest & scikit-learn & 0.24.2 \\
     Support Vector Regressor & scikit-learn & 0.24.2 \\
     K-Nearest Neighbor & scikit-learn & 0.24.2 \\
     AdaBoost Regressor & scikit-learn & 0.24.2 \\
     Neural Network & scikit-learn & 0.24.2 \\
     \midrule
     Auto-Sklearn & auto-sklearn & 0.14.7 \\
     Autogluon & autogluon & 0.5.1 \\
     Flaml & flaml & 1.0.13 \\
     \bottomrule
    \end{tabular}
\end{table*}

%\clearpage
\subsection*{Figures}
\label{app:figures}
\begin{figure*}
\centering
    \includegraphics[height=0.9\textheight]{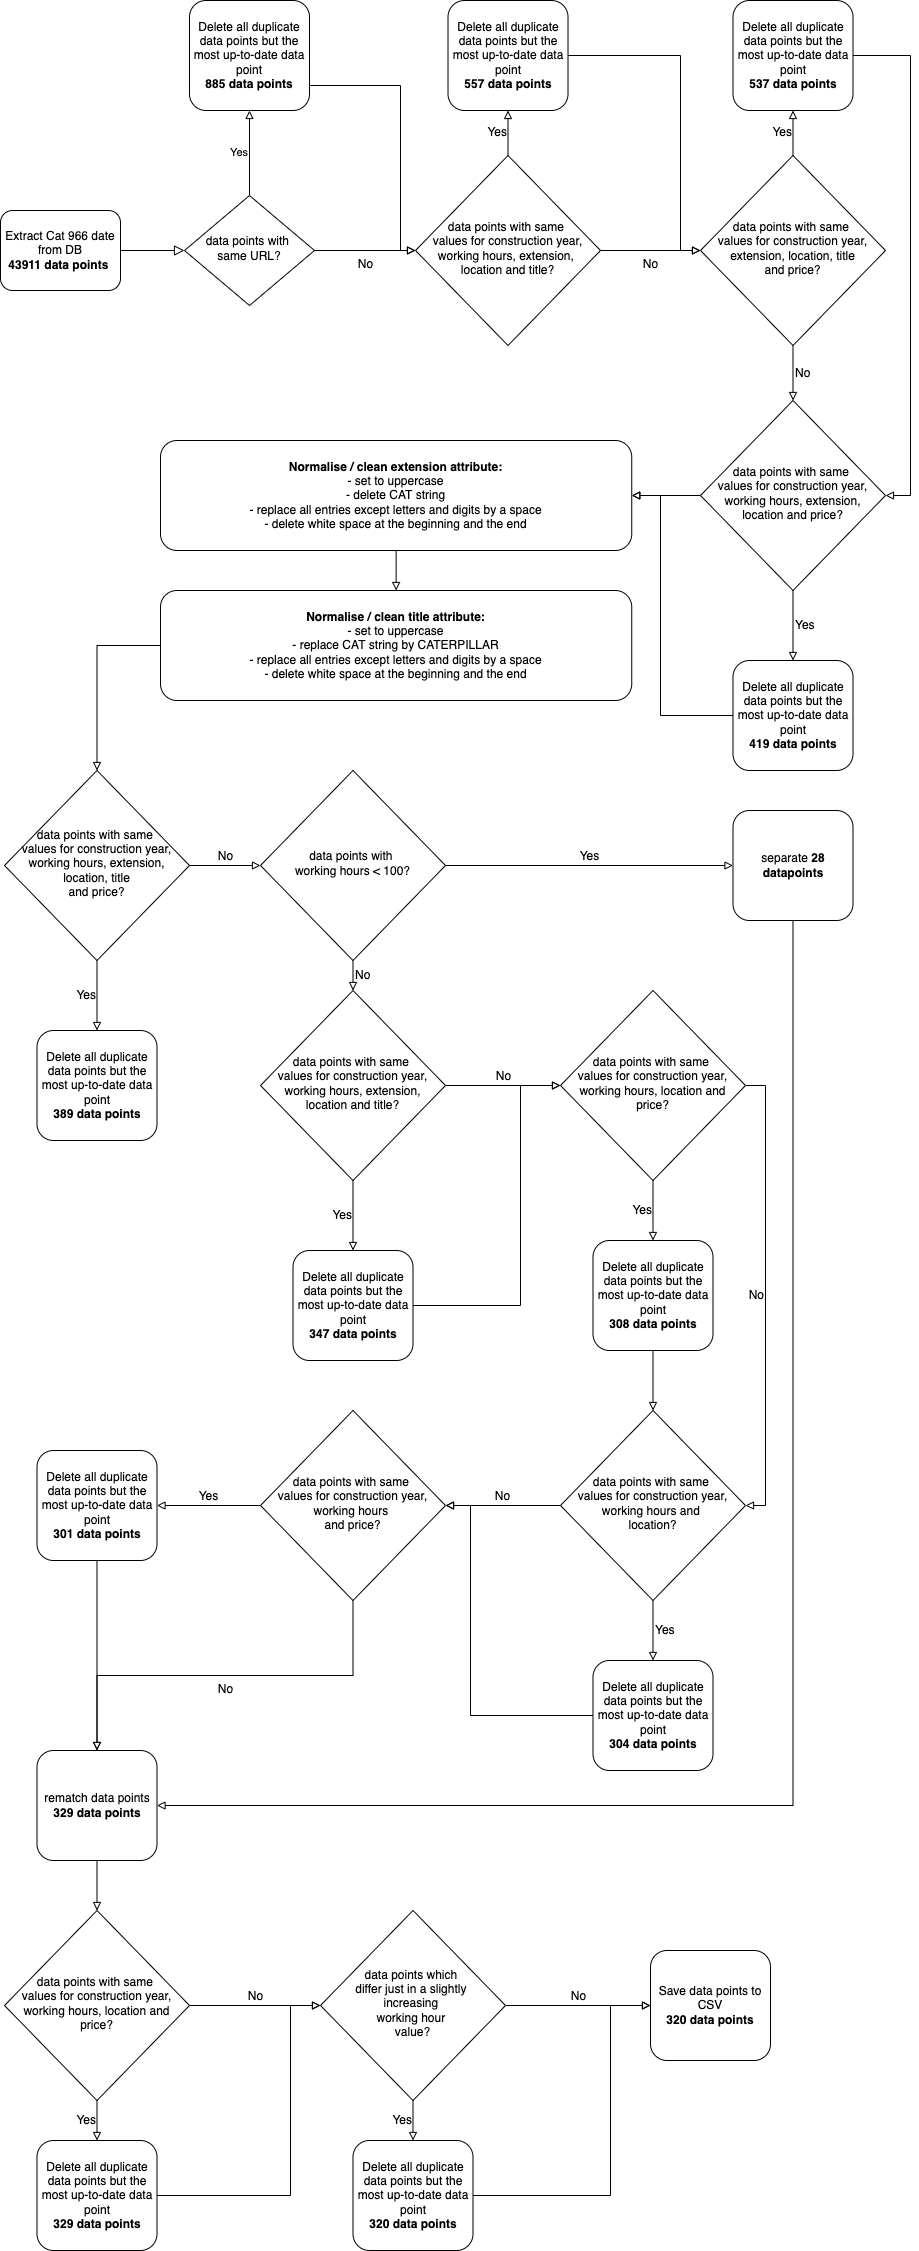}
  \caption{Duplicate detection for the Caterpillar 966}
  \label{fig:dublicate-detection}
\end{figure*}
